# Supplementary material for: Regularized Multi-LLMs Collaboration for Enhanced Score-based Causal Discovery
Source: arXiv:2411.17989 source file (2024-11-27)
Supplement: Supplementary file 1 [file appendix.tex]

\appendix
\section{Appendix}

\subsection{ChatGPT 3.5 results}

\subsubsection{LUCAS}
\begin{center}
    \includegraphics[width = 8cm]{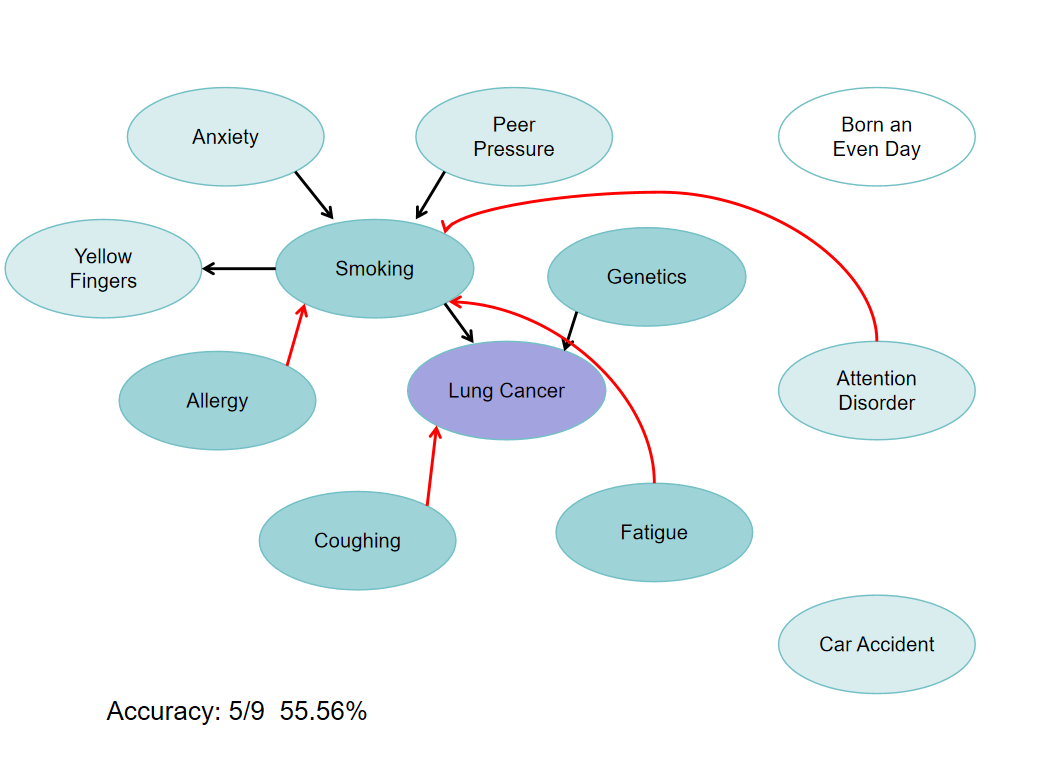}
\end{center}
\subsubsection{Asia}
\begin{center}
    \includegraphics[width = 8cm]{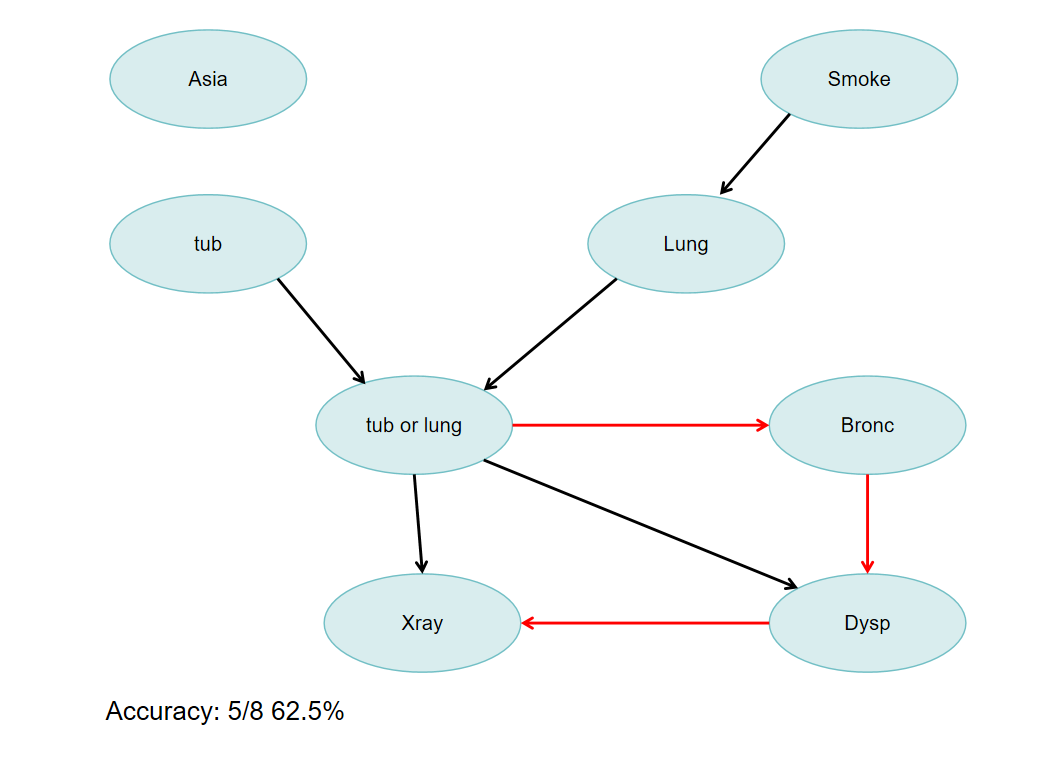}
\end{center}
\subsubsection{SACHS}
\begin{center}
    \includegraphics[width = 8cm]{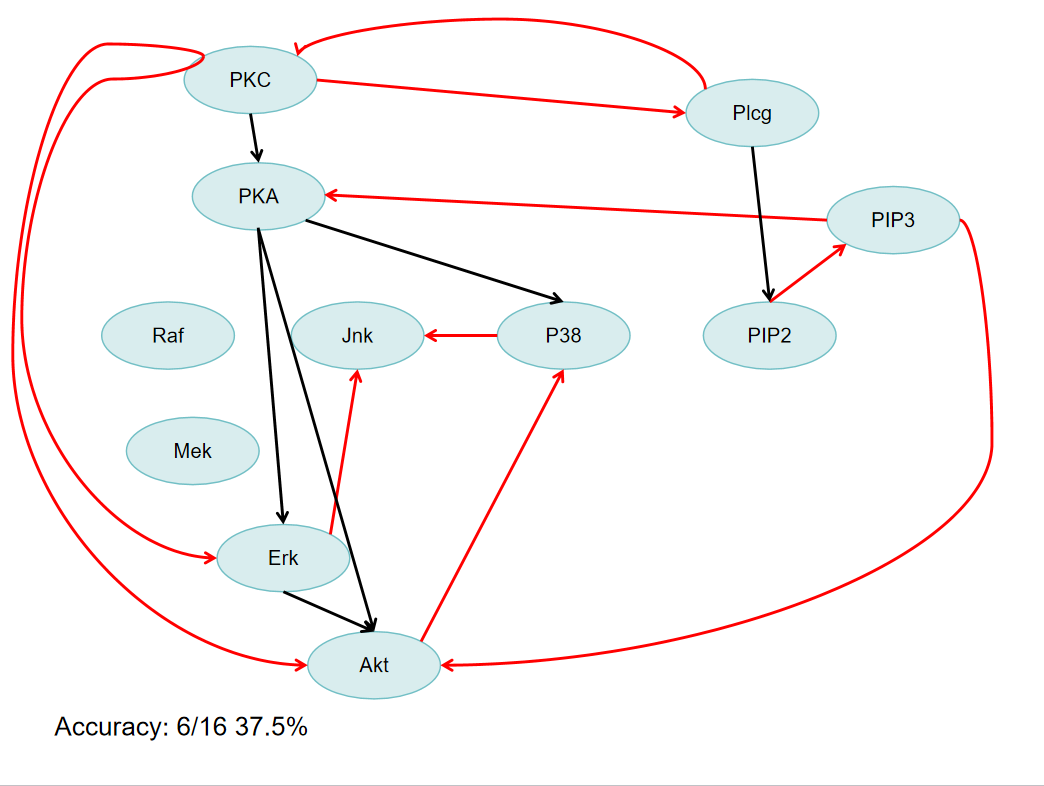}
\end{center}

\subsection{ChatGPT 4 results}
\subsubsection{LUCAS}
\begin{center}
    \includegraphics[width = 8cm]{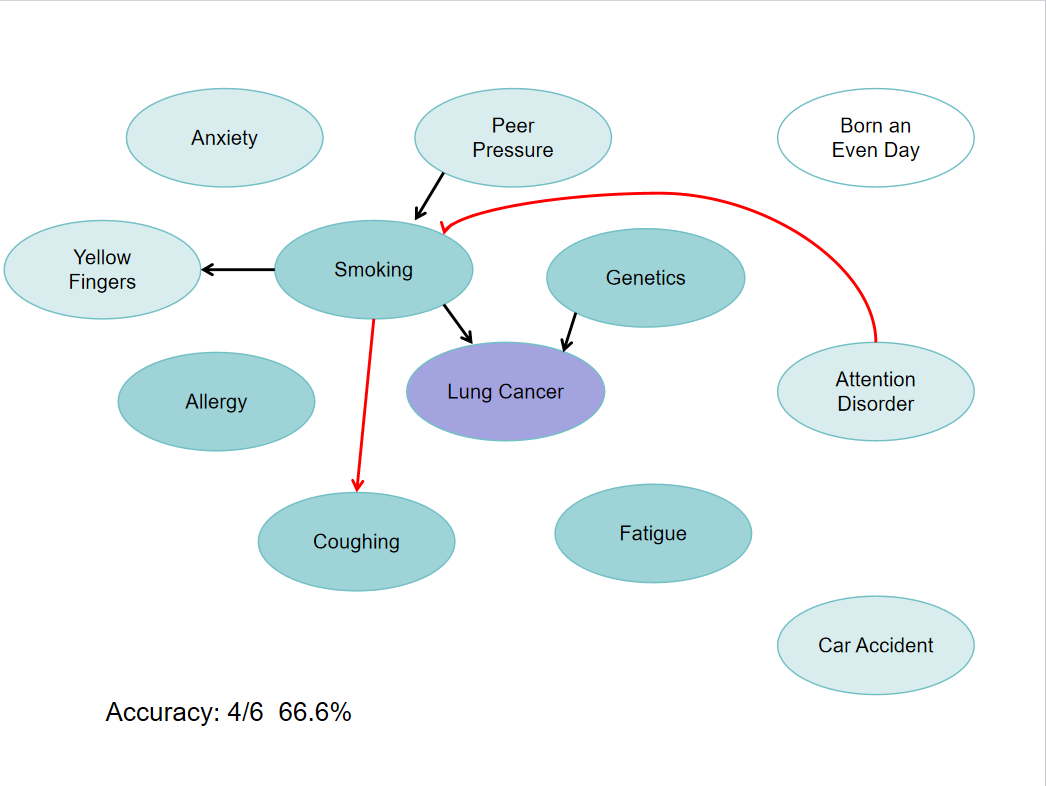}
\end{center}
\subsubsection{Asia}
\begin{center}
    \includegraphics[width = 8cm]{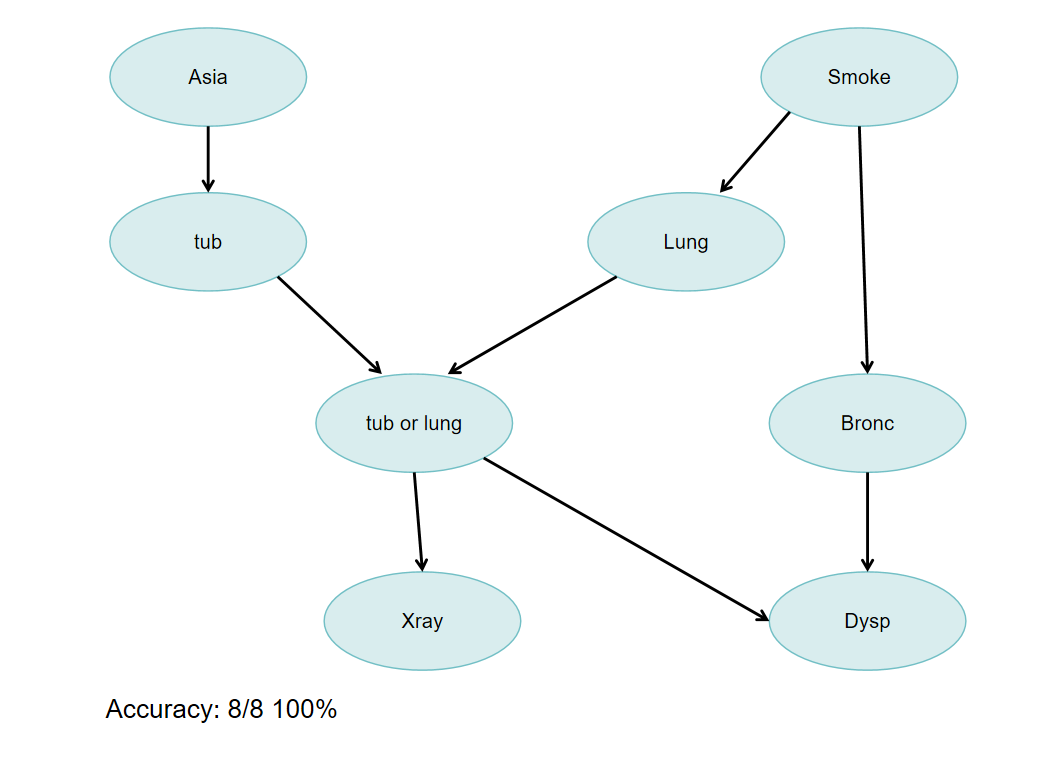}
\end{center}
\subsubsection{SACHS}
\begin{center}
    \includegraphics[width = 8cm]{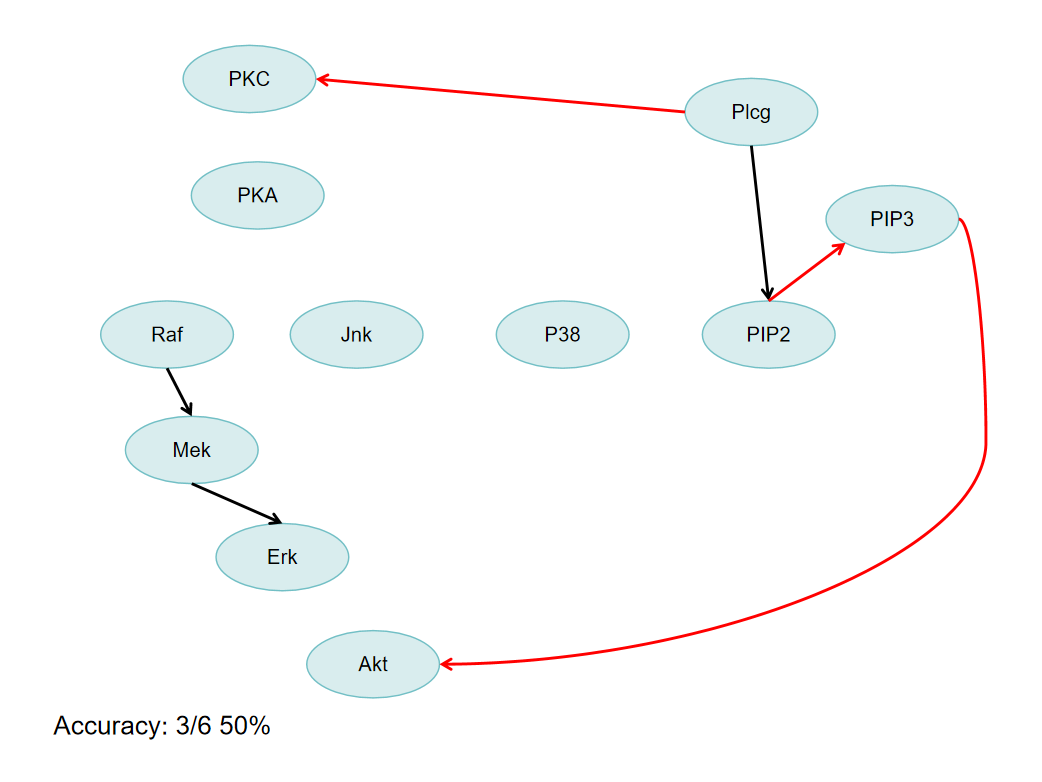}
\end{center}

\subsection{Gemini results}
\subsubsection{LUCAS}
\begin{center}
    \includegraphics[width = 8cm]{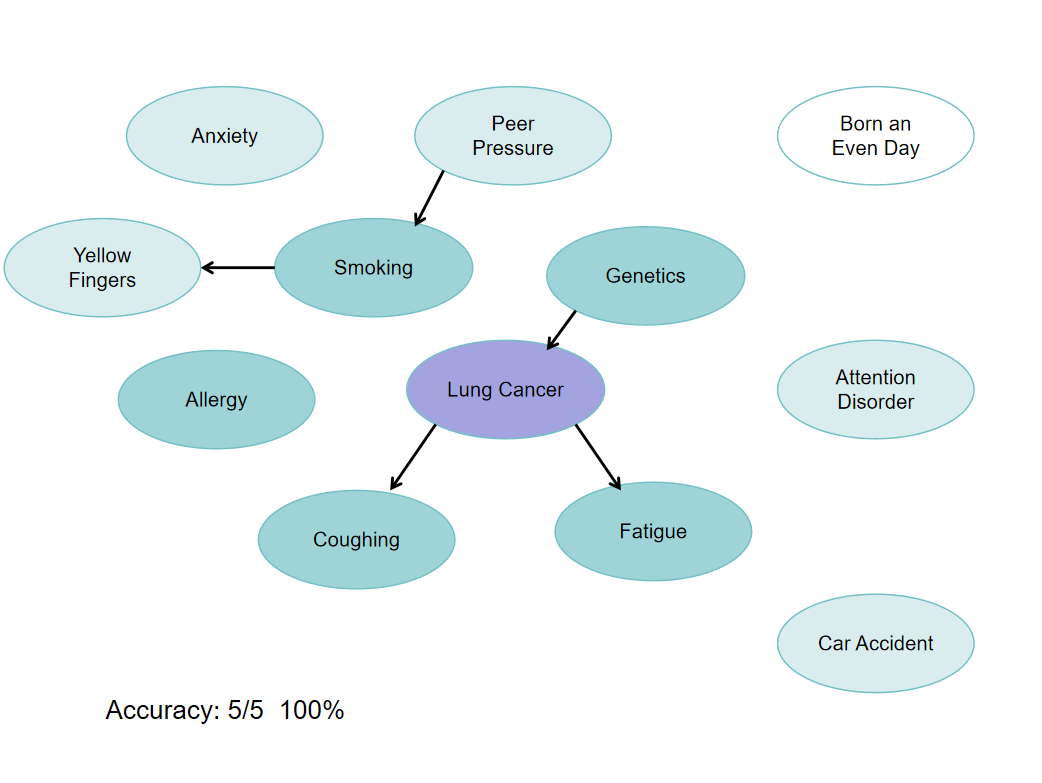}
\end{center}
\subsubsection{Asia}
\begin{center}
    \includegraphics[width = 8cm]{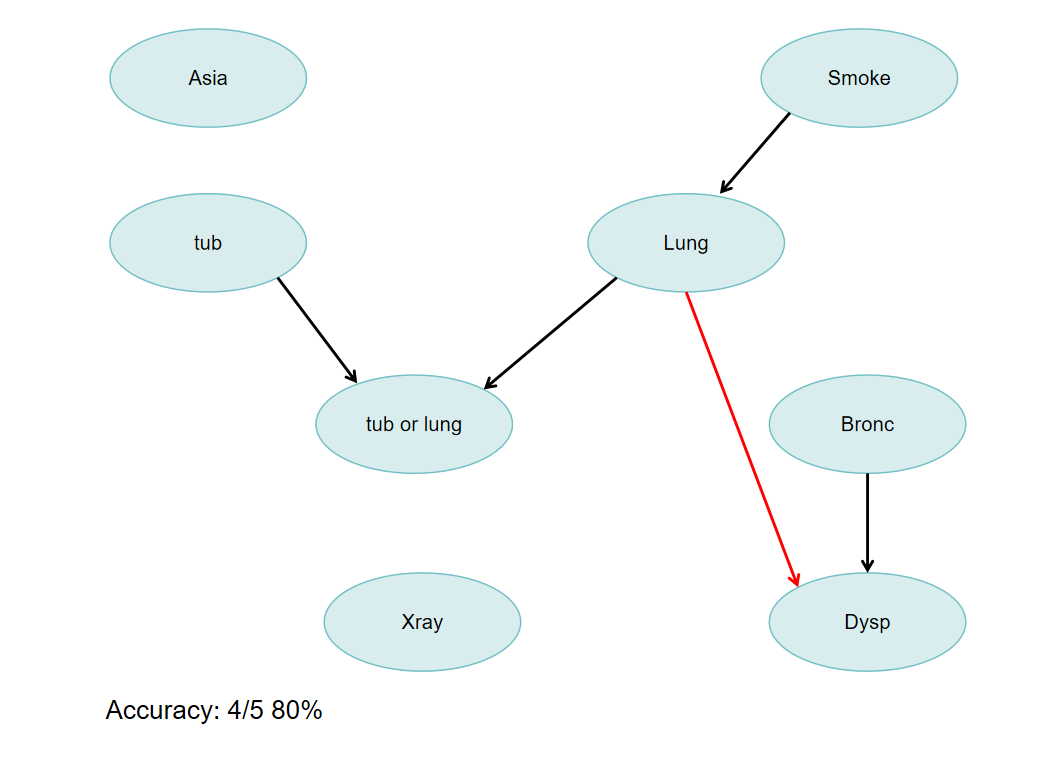}
\end{center}
\subsubsection{SACHS}
\begin{center}
    \includegraphics[width = 8cm]{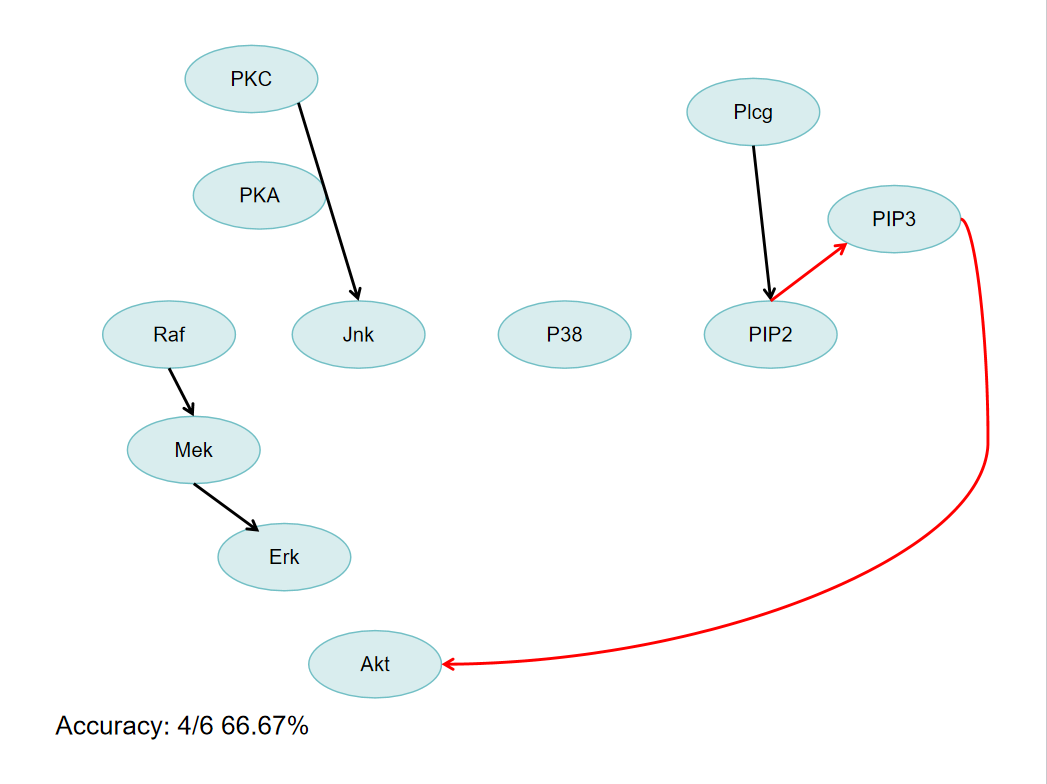}
\end{center}

\subsection{Gemma results}
\subsubsection{LUCAS}
\subsubsection{Asia}
\subsubsection{SACHS}
